# Supplementary material for: Unidirectional propagation of spin waves excited by femtosecond laser pulses in a planar waveguide
Source: arXiv:2209.05611 ancillary file (2023-02-28)
Supplement: Supplementary file 1 [file SW_in_waveguides_Suppl_Mat.pdf]

# Unidirectional propagation of spin waves excited by femtosecond laser pulses in a planar waveguide: Supplementary Materials

P. I. Gerevenkov,* Ia. A. Filatov, A. M. Kalashnikova, and N. E. Khokhlov

*Ioffe Institute, 194021 St. Petersburg, Russia*

(Dated: February 28, 2023)

# I. EXCITATION REALIZATION

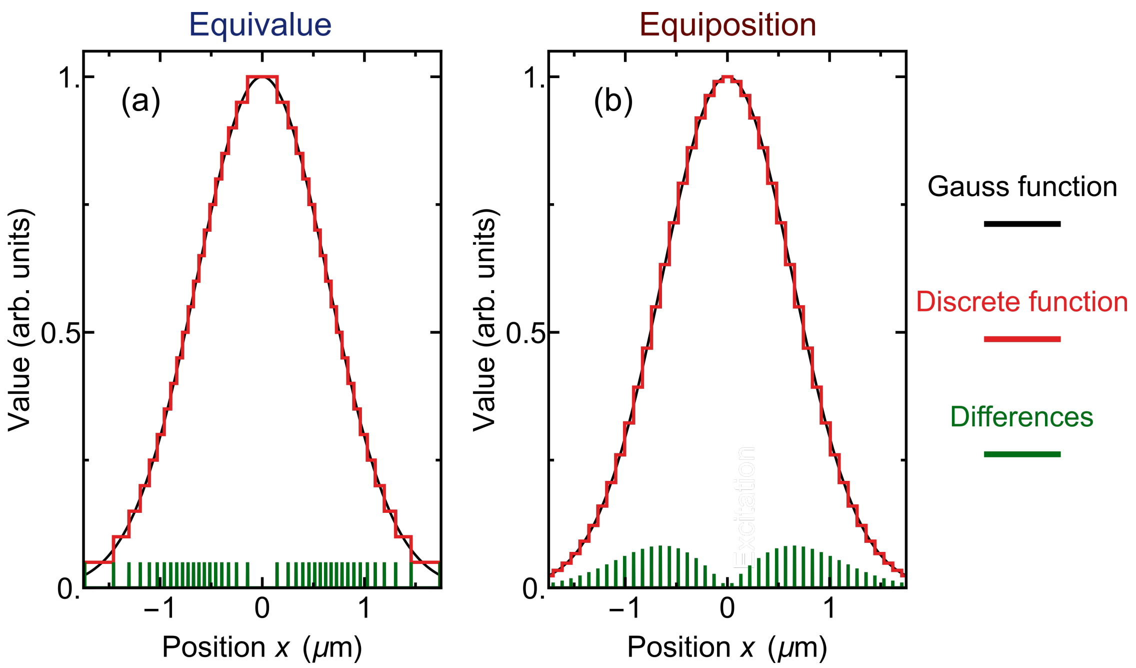


FIG. S.1. The form of the Gaussian distribution (red line) in the case of discretization by the values of the function (a) and by the values of the parameter (b). The corresponding differences shown by green line. Black solid line shows the continuous Gaussian distribution. The dependencies are given for $imax = 20$ for clarity.

Since the mumax$^3$ does not allow introducing a continuous change in the magnetic parameters, a discrete Gaussian function was used for excitation area. To minimize abrupt changes in parameters, we used discretization by function values. In this case, the resulting surges have the same values, in contrast to the case of parameter discretization (see Fig. S.1). When comparing the differences (green line in Fig. S.1), it can be seen that in the case of discretization by the argument, the values of the jumps reach almost twice as large as in the case of discretization by values. Large values of a sharp magnetic parameters change lead to the excitation of exchange waves, which are not observed in experiments of optical MSWs excitation by a laser-induced anisotropy change [1, 2]. In the model, the excitation area realized as follows:

* petr.gerevenkov@mail.ioffe.ru; http://www.ioffe.ru/ferrolab/

```
imax := 64 // number of pumped regions
//  region imax (not pumped)
c := cuboid(sizeX, sizeY, sizeZ)
DefRegion(imax, c)

//  pumped region
pumpSize := (1.5e-6)/2.355 // (pump FWHM) / 2.355 eq gauss sigma
// set pump region with gaussian shape
for i := 1; i < imax; i++{
    a0 := 1-(i-1)/imax
    a1 := 1-i/imax
    a := cylinder(sqrt(2*pow(pumpSize,2)*Log(1/a1)), sizeZ).
        transl(Pump_x_position, 0, 0 )
    b := cylinder(sqrt(2*pow(pumpSize,2)*Log(1/a0)), sizeZ).
        transl(Pump_x_position, 0, 0 )
    DefRegion(i, c.intersect(a.sub(b)))
    Msat.setregion(i, Msat_Py) // Magnetization saturation [A/m]
    alpha.setregion(i, alpha_Py) // Gilbert damping constant
    Ku1.setregion(i, Ku1_Py) // Uniaxial anizotropy contant [J/m3]
    Aex.setregion(i, A_ex_Py) // Exchange stiffnes [J/m]
    anisU.setregion(i, vector(sin(AnizotropyDir), cos(AnizotropyDir), 0))
}
```

where $imax$ – discretization parameter (on Fig. S.1 $imax = 20$ for clarity); $sizeX$, $sizeY$ and $sizeZ$ are waveguide sizes; $Pump\_x\_position = x_0$; $Msat\_Py$, $alpha\_Py$, $Ku1\_Py$ and $A\_ex\_Py$ – saturation magnetization, Gilbert damping parameter, anisotropy parameter and exchange stiffness parameter values before the excitation. Next, we run simulations for $timeBeforeStart = 0.5$ ns to verify that there is no magnetic dynamics caused by incomplete relaxation to the equilibrium state. This period is shown on all time dependences as a signal at $t < 0$. After that excitation was performed:

```
// set pump region parameters
for i:=1; i<imax; i++{
    a0 := 1-(i-1)/imax
    a1 := 1-i/imax
    //  magnetic parameters after laser-induced heating
    Msat.setregion(i,(1-((a1+a0)/2)*0.1*
        pow(2.718,-3.3*(t-timeBeforeStart)*10e9))*Msat_Py)
        // Magnetization saturation [A/m]
    Ku1.setregion(i,pow((1-((a1+a0)/2)*0.1*
        pow(2.718,-3.3*(t-timeBeforeStart)*10e9)),3)*Ku1_Py)
        // Cubic anizotropy contant [J/m3]
}
```

## II. DETECTION REALIZATION

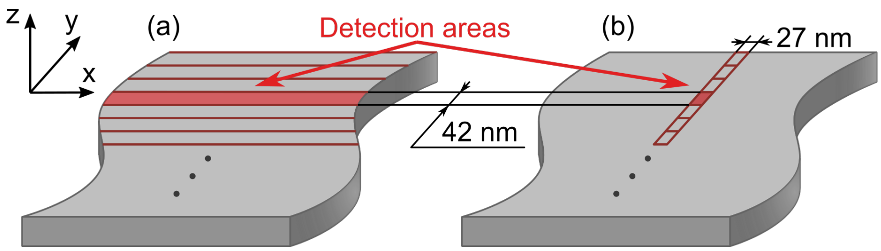


FIG. S.2. Schematic illustration of detection regions in the experiments of uniform (a) and spot (b) excitation.

In the simulations of uniform excitation the detection is organized as follows: the instantaneous values of the magnetization components are averaged over the regions of full waveguide length and 8 cells (or 42 nm) width (see Fig. S.2 a). In this cases the increasing of damping parameter close to $y$-edges is not used.

In the simulations of elongated and round spot excitation the magnetization components are averaged over the regions of 8 cells (or 27 nm) length and 8 cells (or 42 nm) width, located at a distance $y_d$ =10.5 $\mu$m from the excitation area (see Fig. S.2 b). In all experiments we use 128 detection areas across the waveguide.

## III. STATIC MAGNETIZATION DISTRIBUTIONS

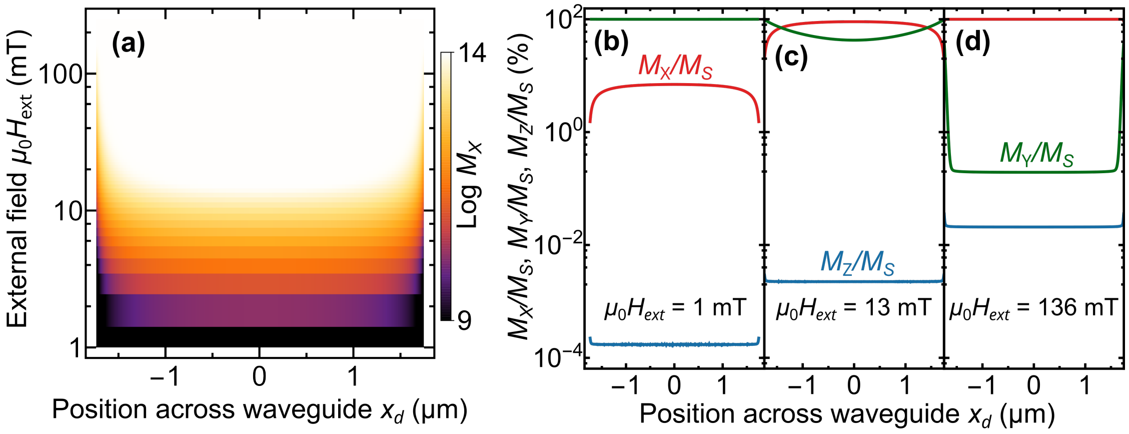


FIG. S.3. (a) Dependence of equilibrium $M_X$ distribution across waveguide as a function of external magnetic field. (b-d) $M_X$, $M_Y$ and $M_Z$ equilibrium magnetization components distribution across waveguide at $\mu_0 H_{ext} = 1$, 13 and 136 mT, respectively. All dependences are presented for an unheated waveguide.

Figure S.3 a shows the static magnetization component along the external magnetic field as a function of $x_d$ and $H_{ext}$. Demagnetizing fields lead to a difference in saturation field values for the center and edges of the waveguide. For the waveguide center $x_d = 0\,\mu$m, the magnetization saturates above 20 mT, while the edges saturate above 200 mT (white color in Fig. S.3 a).

At $\mu_0 H_{ext} = 1$ mT (which is much smaller then anisotropy field over the entire waveguide width), the magnetization is directed along the anisotropy axis, i.e. along $y$ direction (see Fig. S.3 b). At $\mu_0 H_{ext} = 13$ mT the magnetization direction is close to the $x$ axis in the waveguide center and still along the $y$ axis at the edges (see Fig. S.3 c). For $\mu_0 H_{ext} = 136$ mT the $M_Y/M_S$ and $M_Z/M_S$ are less than 1 % everywhere except the regions near the waveguide edges (see Fig. S.3 d).

## IV. AMPLITUDES IN THE CASE OF UNIFORM EXCITATION

Figure S.4 a shows the impact of a laser pulse on the magnetic parameters ($K_U$ and $M_S$). Figures S.4 b and c on the same timescale show the dynamics of $M_Z$ magnetization

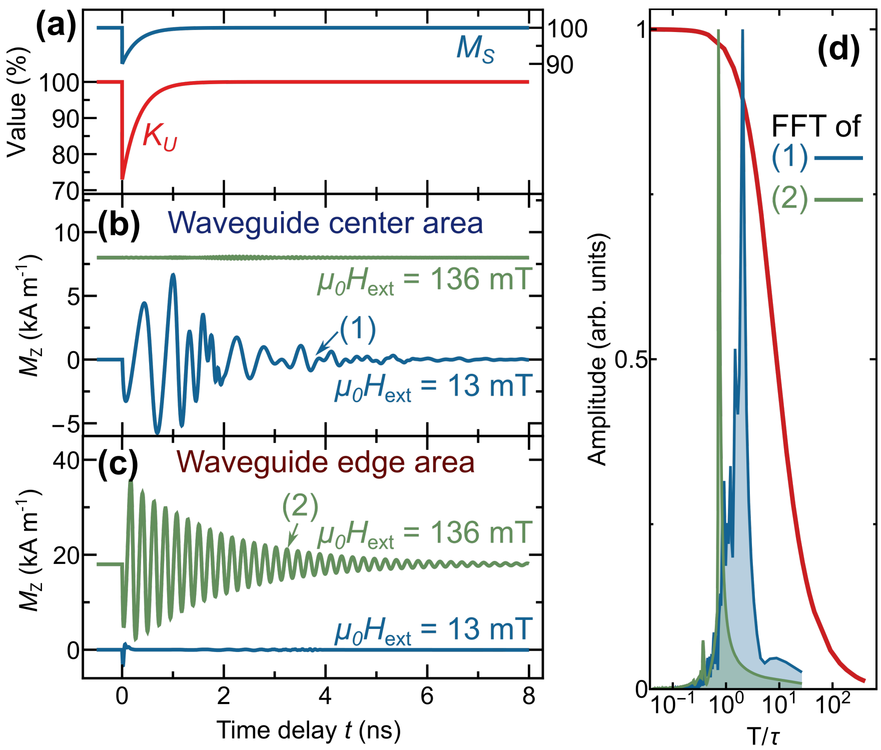


FIG. S.4. (a) Temporal dependencies of magnetic parameters $K_U$ and $M_S$. Temporal dependencies of excited $M_Z$ magnetization component dynamics at the center (b) and at the edge (c) of the waveguide. The signals are presented for $\mu_0 H_{ext} = 13$ and 136 mT in the case of uniform excitation of the entire waveguide area. The initial state $M_Z(t < 0) = 0$ in all cases, an additional shift is introduced for clarity. (d) Normalized excited precession amplitude as a function of the $T/\tau$ ratio (solid red line) obtained using Eq. S.1 and normalized FFT spectra of signals (1) from (b) and (2) from (c).

component at the center and at the edge of the waveguide at $\mu_0 H_{ext} = 13$ and 136 mT in the case of uniform excitation. It can be seen that the dynamics in the center and at the edge are excited more efficiently in a field of 13 and 136 mT, respectively (lines marked 1 and 2). Herewith, the precession frequency is higher at the waveguide edge due to the contribution of uncompensated uniaxial anisotropy. To determine the effect of ratio between precession period $T$ and magnetic parameters relaxation time $\tau$ on the excitation efficiency, we perform the numerical solution of Landau–Lifshitz equation:

$$\frac{\partial \mathbf{m}}{\partial t} = -|\gamma| \left[ \mathbf{m} \times \left( -\frac{1}{M_S} \frac{\partial F_{tot}}{\partial \mathbf{m}} \right) \right], \tag{S.1}$$

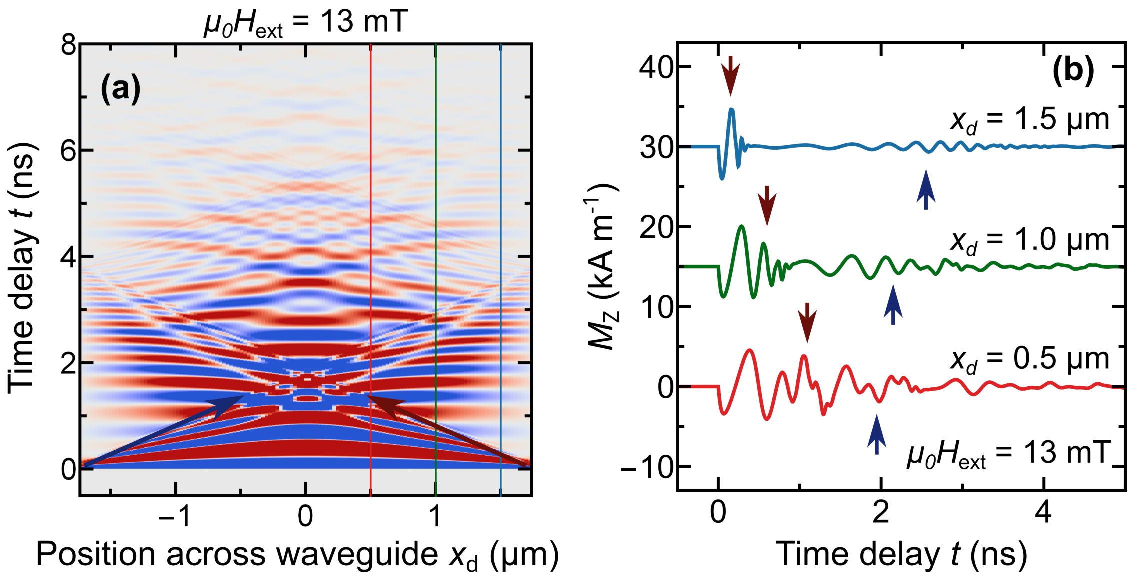


FIG. S.5. (a) Magnetization dynamics signal as a function of time delay and $x_d$. The propagating SWs marked by arrows. (b) Precession signals containing wave packets of propagading SWs for various positions across waveguide. The corresponding positions in (a) marked by lines. The red down and blue up arrows marks the wave packets propagates from edges at $x_d = 1.75$ and -1.75 $\mu$m, respectively. The initial state $M_Z(t < 0) = 0$ in all cases, an additional shift is introduced for clarity.

where $\mathbf{m} = \{m_X, m_Y, m_Z\} = \mathbf{M}/M_S$, $F_{tot} = F_A + F_H + F_M$ is free energy density, which consist of anisotropy: $F_A = -K_U {m_Y}^2$, Zeemann: $F_H = -\mu_0 M_S m_X H_{ext}$ and dipole: $F_M = \frac{1}{2}\mu_0 {M_S}^2 {m_Z}^2$ contributions.

The initial state is defined as

$$\frac{\partial F_{tot}}{\partial \mathbf{m}} = 0, \text{ at } t < 0. \tag{S.2}$$

When solving equation S.1, the value $\mu_0 H_{ext} = 9$ mT was used, and $\tau$ varied in the range from $10^{-2}$ to $10^3$ ns. Figure S.4 d shows the dependence of the excited precession amplitude on $T/\tau$. The data demonstrate that the maximum amplitude is excited when $\tau >> T$. This feature can be explain by overlap area of the spectra of excited precession and excitation force as described in details elsewhere [3]. Comparison of the precession spectra in the center and at the edge of the waveguide (FFT of 1 and 2 on Fig. S.4 d) with this dependence demonstrates amplitude suppression in a field of 13 mT, which explains the different peak

ratios in Fig 2 c and Fig 3 e in the main text.

Even in the case of uniform waveguide excitation, there are waves propagating from the edges due to the magnetic inhomogeneity, as demonstrated in [4–7]. Figure S.5 a shows the dynamics of $M_Z$ magnetization component as a function of time delay and $x_d$. The propagating SWs are marked by arrows. After excitation, the waves propagate across waveguide and are repeatedly reflected from the edges. Precession signals containing wave packets of propagading SWs for various positions across waveguide are shown in Fig. S.5 b. The wave packets propagating from the edges at $x_d = 1.75$ and -1.75 $\mu$m are marked by a red down and a blue up arrows, respectively. The corresponding magnetization dynamics signal at the waveguide center is shown in Fig. 3 b in the main text. SWs propagation and interference result in a complex signal spectrum, so we used the area under the FFT as an estimate of the signal amplitude.

## V. ROUND SPOT EXCITATION IN THE WAVEGUIDE CENTER

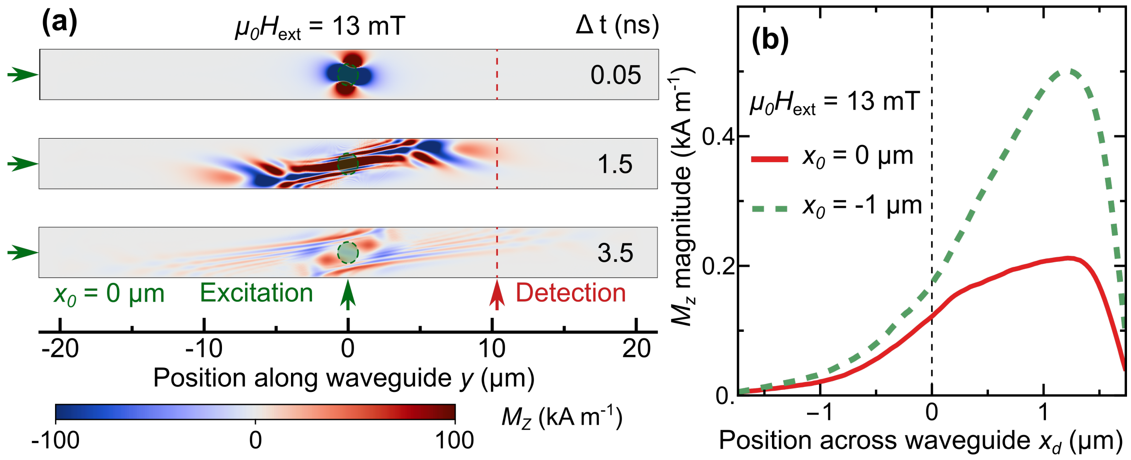


FIG. S.6. (a) distribution of $M_Z$ magnetization component at various times after excitation for $\mu_0 H_{ext} = 13\,\mathrm{mT}$ and $x_0 = 0\,\mu\mathrm{m}$. (b) MSWs magnitudes vs $x_d$ at a distance $y_d = 10.5\,\mu\mathrm{m}$ from the excitation region. Data are given for two positions of excitation $x_0 = 0\,\mu\mathrm{m}$ (solid red line) and $x_0 = -1\,\mu\mathrm{m}$ (dashed green line).

When a round excitation spot is placed at the waveguide center at $\mu_0 H_{ext} = 13\,\mathrm{mT}$, the bidirectional MSWs propagation is observed (see Fig. S.6 a). These waves propagate at the same angle relative to the $y$ axis as in case of elongated spot excitation, but the signal

magnitude is suppressed compared to excitation at $x_0 = -1$ and elongated spot excitation. Comparison of the wave magnitudes vs $x_d$ for $x_0 = 0$ and -1 $\mu$m is shown in Fig. S.6 b.

---


[1] N. E. Khokhlov, P. I. Gerevenkov, L. A. Shelukhin, A. V. Azovtsev, N. A. Pertsev, M. Wang, A. W. Rushforth, A. V. Scherbakov, and A. M. Kalashnikova, Optical excitation of propagating magnetostatic waves in an epitaxial galfenol film by ultrafast magnetic anisotropy change, Physical Review Applied **12**, 044044 (2019).

[2] I. A. Filatov, P. I. Gerevenkov, M. Wang, A. W. Rushforth, A. M. Kalashnikova, and N. E. Khokhlov, Spectrum evolution and chirping of laser-induced spin wave packets in thin iron films, Applied Physics Letters **120**, 112404 (2022).

[3] J. Li, C.-J. Yang, R. Mondal, C. Tzschaschel, and S. Pal, A perspective on nonlinearities in coherent magnetization dynamics, Applied Physics Letters **120**, 050501 (2022).

[4] Y. Au, T. Davison, E. Ahmad, P. S. Keatley, R. Hicken, and V. Kruglyak, Excitation of propagating spin waves with global uniform microwave fields, Applied Physics Letters **98**, 122506 (2011).

[5] C. Davies and V. Kruglyak, Generation of propagating spin waves from edges of magnetic nanostructures pumped by uniform microwave magnetic field, IEEE Transactions on Magnetics **52**, 1 (2016).

[6] N. Träger, P. Gruszecki, F. Lisiecki, F. Groß, J. Förster, M. Weigand, H. Głowiński, P. Kuświk, J. Dubowik, M. Krawczyk, and J. Gräfe, Demonstration of k-vector selective microscopy for nanoscale mapping of higher order spin wave modes, Nanoscale **12**, 17238 (2020).

[7] N. Träger, F. Lisiecki, R. Lawitzki, M. Weigand, H. Głowiński, G. Schütz, G. Schmitz, P. Kuświk, M. Krawczyk, J. Gräfe, and P. Gruszecki, Competing spin wave emission mechanisms revealed by time-resolved x-ray microscopy, Phys. Rev. B **103**, 014430 (2021).
